# Supplementary material for: Hardware-Aware Static Optimization of Hyperdimensional Computations
Source: arXiv:2304.03335 source file (2024-02-20)
Supplement: Supplementary file 1 [file appendix.tex]

\appendix

\section{Data Structures and Dynamic Analysis}
\begin{figure}
\includegraphics[width=0.6\linewidth]{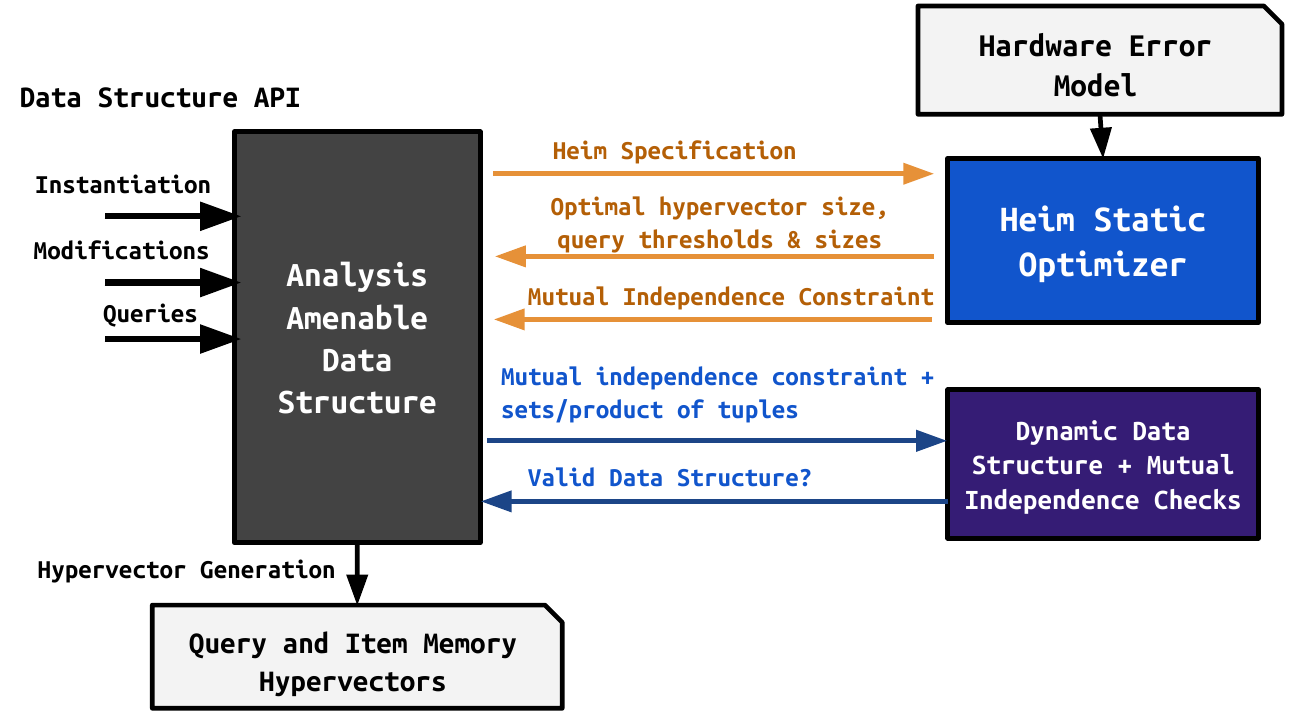}
\caption{data structure overview. \swatch{orange} arrows are static checks, \swatch{blue} arrows are dynamic checks, \swatch{black} arrows are API calls.}
\label{fig:datastruct}
\end{figure}

Figure~\ref{fig:datastruct} presents a visualization of the interactions between the static optimizer, the analysis amenable data structure, and the mutual independence checker.

\section{Analysis-Amenable Data Structures}\label{sec:datastructure:appendix}

For each data structure, we overview the data structure API and correspond \tool{} specification fragments, and describe the optimizations that are performed to ensure resource-efficient mapping of data structures to hypervectors, and describe the validity checks that are used to ensure data structure integrity. 

\subsection{Mutual Independence Checking Algorithm}\label{sec:dynanalysis:dyncheck}

The \tool{} analysis requires that concrete HD expressions contain \textit{mutually independent} tuples or codes. Intuitively, a set of elements is mutually independent if the existence of each element in the set does not depend on the existence of other elements in the set. Because this sort of check can only be performed over concrete HD expressions, \tool{} also deploys a dynamic checking algorithm that can be used to check if a set of elements is mutually independent.

\noindent\textbf{Algorithm.} We present an efficient dynamic checking algorithm for validating mutual independence of products and sets of tuples. Since the definition of product independence is derived from set independence, if we are able to effectively check set independence, we can also check product independence.
One way to check set independence is exhaustive search, but it is time-consuming, so we derive an equivalent condition that can be efficiently checked.
Given a tuple set $\expr=\sum_{i=1}^nt_i$, denote $c_1,c_2,\cdots,c_m$ as the $m$ relevant codes in $\expr$.
For each tuple $s_i,1\le i\le n$ in $\expr$, we create a binary vector $V_i$ of length $m$, where the $j$-th element is $1$ if $c_j$ is a component of $t_i$, and $0$ otherwise.
The equivalent condition of independence of set $\expr=\sum_{i=1}^nt_i$ is that $V_1,V_2,\cdots,V_n$ are linearly independent in $GF(2)$.
In other words, if we make a $n\times m$ matrix, where the $i$-th row is $V_i$, the equivalent condition is that the matrix's rank is $n$ in $GF(2)$.
For example, for $\expr=a\hdtimes c\hdplus b\hdtimes c\hdplus a\hdtimes b$, if $c_1,c_2,c_3$ are $a,b,c$ respectively, the vectors for $a\hdtimes c,b\hdtimes c,a\hdtimes b$ are $[1,0,1],[0,1,1],[1,1,0]$ respectively.
These $3$ vectors are not linearly independent because $[1,0,1]+[0,1,1]=[1,1,0]$ in $GF(2)$, so $\expr$ is not an independent set.
Intuitively, this is because the binary vector addition in $GF(2)$ represents the binding of tuples, e.g., $1+1=0$ in the previous example's last vector element is because binding $a\hdtimes c$ and $b\hdtimes c$ cancels out $c$.
One can prove that when $V_i,1\le i\le n$ are linearly independent in $GF(2)$, the $t_i,1\le i\le n$ can be viewed as $n$ independently randomly generated hypervectors.
We omit the proof here due to space limit.

Calculating the rank of a $n\times m$ matrix can use a $O(n^2m)$ Gaussian elimination algorithm, which should be sufficiently fast for most HD computations.

\subsection{Set Data Structure}\label{sec:datastructure:set}
\begin{table}[t]
\small 
\begin{tabular}{llll}
\textbf{Set / API call} & \textbf{type} & \textbf{description} & \textbf{\tool{} specification fragment}\\
\hline
\codein{\lit{Set}(M,HDExpr)} & ctor & instantiate set & \codein{\lit{data} \syn{ds} = \lit{sum}(M,HDExpr)}\\
\codein{\lit{add}(query)} & modify & add element to set & \\
\codein{\lit{inSet}(query,acc,fp,fn)} & query & element in set & \codein{\lit{require-accuracy}(VarExpr,\syn{ds},1,acc,fp,fn)}\\
\codein{\lit{subset}(query,M',K,acc,fp,fn)} & query & subset in set & 
\codein{\lit{require-accuracy}(\lit{sum}(M',HDExpr),\syn{ds},K,acc,fp,fn)}\\
&&&\codein{\lit{require-accuracy}(\lit{sum}(M'-1,HDExpr),\syn{ds},K,acc,fp,fn)}\\
&&&\codein{...}\\
&&&\codein{\lit{require-accuracy}(\lit{sum}(K,HDExpr),\syn{ds},K,acc,fp,fn)}\\
\hline

\end{tabular}
\caption{Set API and \tool{} specification fragments. \codein{HDExpr} is a \tool{} abstract HD expression from the grammar in Figure~\ref{fig:grammar:speclang}, \codein{query} is a concrete HD expression in \codein{HDExpr}, \codein{M} is the maximum size of the Set data structure, \codein{M'} is the maximum size of the subset query, and \codein{K} is the number of subset elements to match. The \codein{acc}, \codein{fp}, \codein{fn} rates are the accuracy, false positive, and false negative rates for the query respectively.}
\label{fig:datastruct:set}
\end{table}

Figure~\ref{fig:datastruct:set} presents the analysis-amenable set data structure API and corresponding \tool{} specification fragments. The Set constructor instantiates the abstract data structure in the \tool{} specification, and the data structure queries introduce accuracy requirements into the specification. 

\noindent\textbf{Validity Checks.} The Set data structure ensures that all elements are members of the abstract HD expression \codein{HDExpr} provided to the set constructor. The Set data structure also ensures all elements in the set are mutually independent -- this constraint is imposed by the \tool{} analysis.

\noindent\textbf{Hypervector and Query Optimization.} The data structure writes a single hypervector to item memory with the optimal hypervector size returned by the \tool{} static optimizer. Each query with an optimal query-specific threshold $\threshold_q$ and size $\hvsize_q$ is lowered to a $\hvsize_q$ dimensional hypervector. The distance is then partially computed over the first $\hvsize_q$ bits of the hypervector and compared with the query threshold $\threshold_q$. For subset queries, the data structure looks up the appropriate threshold and query size for the subset size.

\subsection{Analogical Database Data Structure}\label{sec:datastructure:database}

\begin{table}[t]
\small 
\begin{tabular}{llll}
\textbf{Database / API call} & \textbf{type} & \textbf{description} & \textbf{\tool{} specification fragment}\\
\hline
\codein{\lit{Database}(M,VarExpr,VarExpr')} & ctor & create database & \codein{\syn{ds} = \lit{sum}(M,\lit{prod}(VarExpr,VarExpr'))} \\
& & & \codein{\syn{ds2} = \lit{prod}(\syn{ds},\syn{ds})}\\
& & & \codein{\syn{kv} = \lit{prod}(VarExpr,VarExpr')}\\
& & & \codein{\syn{val2} = \lit{prod}(VarExpr',VarExpr')}\\
\codein{\lit{addRecord(i)}} & modify & add record &  \\
\codein{\lit{addEntry(i,entry)}} & modify & add key-value to record &  \\
\codein{\lit{matches}(pairs,M',K,acc,fp,fn)} & query & find records with $\geq$ K & \codein{\lit{require-accuracy}(\lit{sum}(M',\syn{kv}),\syn{ds},K,acc,fp,fn)}\\
&& query tuple matches&\codein{\lit{require-accuracy}(\lit{sum}(M'-1,\syn{kv}),\syn{ds},K,acc,fp,fn)}\\
&&&...\\
&&&\codein{\lit{require-accuracy}(\lit{sum}(K,\syn{kv}),\syn{ds},K,acc,fp,fn)}\\
\codein{\lit{analogy}(query,acc,fp,fn)} & query & analogical query& \codein{\lit{require-accuracy}(\syn{val2},\syn{ds2},1,acc,fp,fn)}\\

\end{tabular}
\caption{Analogical Database API and \tool{} specification fragments. \codein{VarExpr} and \codein{VarExpr'} are \tool{} key and value abstract HD variables expressions from the grammar in Figure~\ref{fig:grammar:speclang}, \codein{pairs} is a tuple set $\subseteq$ in \codein{\lit{prod}(VarExpr,VarExpr'), \codein{query} is a tuple in \codein{\lit{prod}(VarExpr',VarExpr')}}. The value \codein{M} is the maximum size of the Set data structure, \codein{M'} is the maximum size of the subset query, and \codein{K} is the number of subset elements to match. The \codein{acc}, \codein{fp}, \codein{fn} rates are the accuracy, false positive, and false negative rates for the query respectively. The \codein{edge} query is a concept-relation-interaction tuple.}
\label{fig:datastruct:database}
\end{table}

Karnerva~\cite{kanerva2010we} presented a specialized database query that leverages hyperdimensional computing to compute mappings between analogical structures that can be effectively conducted via HDC. The classic example of such a query is the "dollar price of mexico" query in which each database record is queried to fill in the analogy \codein{us:dollar} as \codein{mexico:?}. 

Figure~\ref{fig:datastruct:database} presents an analysis-amenable analogical database data structure that stores individual database records in item memory. Each database record is a hypervector that encodes a set containing up to \codein{M} key-value tuples, where each key-value tuple is a member of \codein{\lit{prod}(VarExpr,VarExpr')}. The \codein{matches} API call finds the records that match at least \codein{K} of the key-value pairs in \codein{pairs}, and the \code{analogy} query retrieves the value in the record that completes the analogical query \codein{query}.

\noindent\textbf{Validity Checks.} The data structure checks that no key is bound more than once in a single record, and validates the tuples in each record set are mutually independent -- this constraint is imposed by the \tool{} analysis. 

\noindent\textbf{Hypervector Optimization.} the width of the record hypervectors stored in memory are set to the optimal hypervector size. Each database query is configured to use the query-specific threshold and query hypervector size. The \codein{matches} queries are specialized to use the threshold and size that corresponds to the the number of elements in the query set.

\subsection{Non-Deterministic Finite Automata}\label{sec:datastructure:nfa}

\begin{table}[t]
\small 
\begin{tabular}{llll}
\textbf{NFA / API call} & \textbf{type} & \textbf{description} & \textbf{\tool{} specification fragment}\\
\hline
\codein{\lit{NFA}(VarExpr,VarExpr',N)} & ctor & NFA instantiation & \codein{\syn{ds} = \lit{sum}(N,\lit{prod}(VarExpr,VarExpr',\lit{perm}(1,VarExpr)))}\\
\codein{\lit{setTransitions}(transitions)} & modify & set NFA transitions & \\
\codein{\lit{startStates}(states)} & modify & set start states & \codein{\syn{states} = \lit{sum}(|VarExpr|,VarExpr)}\\
\codein{\lit{execute}(sym,acc,fp,fn)} & modify/query & apply symbol & \codein{\syn{states'} = \lit{perm}(-1,\lit{prod}(VarExpr,VarExpr',\syn{ds}))}\\
& & & \codein{\lit{require-accuracy}(VarExpr,\syn{states'},acc,fp,fn)}\\
\end{tabular}
\caption{Non-deterministic Finite Automata (NFA) API and \tool{} specification fragments. The \codein{VarExpr} and \codein{VarExpr'} are \tool{} state and character and HD variable expressions from the grammar in Figure~\ref{fig:grammar:speclang}. \codein{N} is the maximum number state transitions. The \codein{acc}, \codein{fp}, \codein{fn} rates are the accuracy, false positive, and false negative rates for the query respectively.}
\label{table:ds:nfa}
\end{table}

Figure~\ref{table:ds:nfa} presents the API for an analysis-amenable non-deterministic finite automata that is built on the HD finite-state automata formulation developed by Pashchenko et al.~\cite{pashchenko2020search}. The NFA maintains a state hypervector over NFA state codes (\syn{states}) and transition hypervector over state-symbol-state tuples (\syn{ds}). The permutation operator encodes the history of states. The API provides endpoints for instantiating an \codein{N} transition NFA and for instantiating the NFA transitions and inital set of states. The \codein{\lit{execute}} endpoint applies a symbol to the NFA and computes the NFA's next set of states. The execution endpoint qualifies as a query because it ensure the current state can be accurately recovered from the state vector with accuracy \codein{acc}. To generate a \tool{} specification, the NFA execution calls need to be unrolled a fixed number of types.

\noindent\textbf{Validity Checks.} The NFA checks that the start state set is valid - it should only contain mutually independent state codes.

\noindent\textbf{Hypervector Optimization.} The NFA uses the optimal hypervector size for the state and transition hypervectors. The NFA uses the query size and threshold to successively query NFA states and rebuild a lower-noise state vector. This noise-reducing 'cleanup' operation enables the HD computational error to remain relatively controlled as the DFA continues execution. In the event the NFA has a monotonically decreasing set of states, the size of the state vector is dynamically reduced using the query-specific dimension.

\section{Detailed Benchmark Information}\label{sec:benchmarks:detailed}

\begin{figure}
\begin{subfigure}[b]{0.2\textwidth}
\small
\begin{Verbatim}[formatcom=\sffamily,commandchars=\\\{\}]
\lit{int} L = range(\swatch{red},1000,1900)
\lit{Codebook} codes = randCodes(L);
\lit{Set} set = \lit{Set}(500,codes)
for(i in 0...500)
    set.\lit{add}(randCode(\swatch{red},codes))
query = randCode(\swatch{red},codes)
return set.\lit{inSet}(query)
\end{Verbatim}
\label{fig:benchmarks:set}
\caption{\codein{set}}
\end{subfigure}
\hfill
\begin{subfigure}[b]{0.35\textwidth}
\small
\begin{Verbatim}[formatcom=\sffamily,commandchars=\\\{\}]
\lit{Codebook} ks = randCodes(100)
\lit{Codebook} vs = randCodes(101)
\lit{Database} db = \lit{Database}(100,ks,vs)
\lit{int} mn = range(\swatch{red},1,19)
db.\lit{addRecord}(1)
for(i in 1...100)
    db.\lit{addEntry}(1,ks[i],vs[i])
db.\lit{addRecord}(2)
for(i in 2...101)
    db.\lit{addEntry}(2,ks[i],vs[i])
query = \{(ks[1],vs[1]),...,(ks[mn],vs[mn])\}
return db.\lit{matches}(query,mn,mn)
\end{Verbatim}
\caption{\codein{db-match}}
\label{fig:benchmarks:database:matching}
\end{subfigure}% 
\begin{subfigure}[b]{0.35\textwidth}
\small
\begin{Verbatim}[formatcom=\sffamily,commandchars=\\\{\}]
\lit{Codebook} keys = randCodes(15)
\lit{int} L = range(\swatch{red},1,20)
\lit{Codebook} vals = randCodes(15*L)
\lit{Database} db = \lit{Database}(15,keys,vals)
for(i in 1...L)
    db.\lit{addRecord}(i)
    for(j in 1...15)
        db.\lit{addEntry}(i,keys[j],vals[(i-1)*15+j])
return db.\lit{analogy}(\swatch{red})
\end{Verbatim}
\caption{\codein{db-analogy}}
\label{fig:benchmarks:database:analogy}
\end{subfigure}

\begin{subfigure}[b]{0.45\textwidth}
\small
\begin{Verbatim}[formatcom=\sffamily,commandchars=\\\{\}]
\lit{int} maxD = range(\swatch{red},4000,36000)
\lit{Codebook} c = randCodes(200)
\lit{Codebook} r = randCodes(5)
\lit{Codebook} in = randCodes(2)
\lit{KG} kg = \lit{KG}(c,r,in,maxD)
for(i in 0...200)
    edges = \{\}
    deg = range(\swatch{red},0,maxD)
    for(j in 0...deg)
        e = (randCode(\swatch{red},c),randCode(\swatch{red},r),randCode(\swatch{red},in))
        edges.add(e)
    kg.\lit{addVertex}(edges)
query = (randCode(\swatch{red},c),randCode(\swatch{red},r),randCode(\swatch{red},in))
return KG.\lit{hasEdge}(query)
\end{Verbatim}
\caption{\codein{graph}}
\label{fig:benchmarks:database:knowledge}
\end{subfigure}%
\begin{subfigure}[b]{0.45\textwidth}
\small
\begin{Verbatim}[formatcom=\sffamily,commandchars=\\\{\}]
\lit{Codebook} c = randCodes(26)
\lit{String} bs = randStr(\swatch{red},20)
\lit{int} bl = len(bs)
\lit{Codebook} s = randCodes(bl+1)
\lit{int} ql = range(\swatch{red},2,10)
\lit{String} qs = randStr(\swatch{red},ql)
\lit{NFA} nfa = \lit{NFA}(s,c,bl)
transitions = \{\}
for(i in 0...bl)
    transitions.add((s[i],bs[i],s[i+1]))
nfa.\lit{setTransitions}(transitions)
nfa.\lit{startStates(s)}
for(i in 0...ql)
    nfa.\lit{execute}(qs[i])
\end{Verbatim}
\caption{\codein{nfa}}
\label{fig:benchmarks:database:nfa}
\end{subfigure}

\caption{Benchmark data structure programs. The \swatch{red} symbols are randomly populated to produce different data structure instantiations.}
\label{fig:benchmarks}
\end{figure}

Figure~\ref{fig:benchmarks} presents the data structure query generation procedures for each of the benchmark applications evaluated in the results section.

\subsection{Benchmark Parametrizations}

We use different benchmark parametrizations so that we observe variations in accuracy and in the optmized parameters. 

\noindent\textbf{Accuracy / Resource Utilization Experiments.} For the accuracy and resource utilization experiments presented in Section~\ref{sec:results:resource}, we use the following benchmark parametrizations.

\begin{itemize}[leftmargin=*,label=$\tinybullet$]
\item\textbf{\codein{set}} (Section~\ref{sec:datastructure:set}) - we construct 1000 random set data structures, each containing 20-200 codes sampled from randomly sampled codebook with 40-400 codes.

\item\textbf{\codein{db-match}.} (Section~\ref{sec:datastructure:database})
We construct 10000 random instantiations of a 2 record, 20 key-value pair database from a codebook of 20 keys and 40 values. The query constructs a random subset of 1-10 key-value pairs and counts the number of record matches in the database. 

\item\textbf{\codein{db-analogy}.} (Section~\ref{sec:datastructure:database}) We construct 10000 random instantiations of a 1-20 record, 15 key database and map each key to a unique value.

\item\textbf{\codein{knowledge-graph}.} (Section~\ref{sec:datastructure:knowledgegraph}) We construct 38000 random instantiations of a 20-vertex, 5-relation knowledge graph with degree of 1-380.

\item\textbf{\codein{nfa}.} (Section~\ref{sec:datastructure:nfa}) We construct 800 nondeterministic finite automatas (NFA) that recognizes strings of length 8. The query operation constructs 2 random query strings with a length of 1-8 and counts the number that are correctly recognized by the NFA.
\end{itemize}

\noindent\textbf{Dynamic Thresholding Comparison.} We use the benchmark parametrizations described below. Generally speaking, the data structures used in this set of experiments are larger, since these executions are working with a fixed 10,000 dimensional hypervector size and need to encode more data to observe accuracy degradations.

\begin{itemize}[leftmargin=*,label=$\tinybullet$]
\item\textbf{\codein{set}.} (Section~\ref{sec:datastructure:set}) We construct 1000 random set data structures, each containing 500 codes sampled from a randomly generated codebook with 1000-19000 codes. The query tests if a random code in codebook is in the set. 

\item\textbf{\codein{db-match}.} (Section~\ref{sec:datastructure:database}) We construct 3000 random instantiations of a 2 record, 100 key-value pair database from a codebook of 100 keys and 100 values. The query constructs a random subset of 1-19 key-value pairs and counts the number of record matches in the database. 

\item\textbf{\codein{db-analogy}.} (Section~\ref{sec:datastructure:database}) We construct 1000 random instantiations of a 10-20 record, 20 key database and map each key to a unique value. The query operation constructs a random analogy query and then tests to see if the database returns the correct value match.

\item\textbf{\codein{knowledge-graph}.} (Section~\ref{sec:datastructure:knowledgegraph}) We construct 10 random instantiations of a 200-vertex, 5-relation knowledge graph with degree of 4000-36000.
For each graph, we randomly generate 100 edge queries and test whether they match with every vertex.

\item\textbf{\codein{nfa}.} (Section~\ref{sec:datastructure:nfa}) We construct 1000  nondeterministic finite automatas (NFA) that recognizes strings of length 20. The query operation constructs 2 random query strings with a length of 2-10 and counts the number that are correctly recognized by the NFA.
\end{itemize}
