# Supplementary material for: Hardware-Aware Static Optimization of Hyperdimensional Computations
Source: arXiv:2304.03335 source file (2024-02-20)
Supplement: Supplementary file 2 [file supplementary.tex]

\section{Supplementary Materials}

\subsection{Analysis-Amenable Data Structures with the Heim Specification Language}\label{sec:datastructures}

We provide a practical analysis-amenable data structure library that uses \tool{}'s static analysis framework to optimize the data structure and query hypervectors and thresholds. Each data structure offers an API for instantiating, adding new elements to, and querying the data structure. Section~\ref{sec:datastructure:knowledgegraph} presents a detailed description of our novel, analysis-amenable knowledge graph formulation. Both the data structure construction operations and data structure queries can be formalized with the \tool{} specification language, and therefore statically optimized with \tool{}'s static optimizer. The analysis-amenable set, NFA, and analogical database data structures are adapted from HD encodings from prior work~\cite{pashchenko2020search,kanerva2010we,gayler1998multiplicative,kleyko2021survey1,kleyko2022vector}, and are presented in Section~\ref{sec:datastructure:set}, \ref{sec:datastructure:database}, \ref{sec:datastructure:nfa} respectively.

\noindent\textbf{Data Structure Usage.} The end user instantiates, modifies, and queries the data structures through the data structure's API. The data structure then translates API calls to a \tool{} accuracy specification that is then solved by the \tool{} static optimizer. The \tool{} static optimizer returns the optimal hypervector size, the collection of query-specific thresholds and sizes to use, and any independence constraints imposed by the analysis. The data structure then uses these parameterization at runtime to optimally generate query hypervectors and data structure hypervectors to store in item memory. Once the item memory is constructed, queries are made against the data structure by constructing query hypervectors and then computing the distance between the query hypervector and all hypervectors in item memory. Each analysis-amenable data structure can be configured to perform runtime checks that ensure the data structure and any associated queries satisfy all independence constraints imposed by \tool{}'s static optimization procedure.

\subsubsection{Knowledge Graph Data Structure}\label{sec:datastructure:knowledgegraph}

\begin{table}[t]
\footnotesize
\setlength{\tabcolsep}{1.5pt}
\begin{tabular}{lllp{5cm}}
\textbf{Knowledge Graph / API call} & \textbf{type} & \textbf{description} & \textbf{\tool{} specification fragment}\\ \hline
\texttt{\lit{KG}(VarExpr,VarExpr',VarExpr'',N)} & ctor & instantiation & \syn{edge} = \lit{prod}(VarExpr,VarExpr',VarExpr'')\\
& & & \syn{ds} = \lit{sum}(N,\syn{edge})\\
\texttt{\lit{addVertex}(edges)} & modify & add vertex & \\
\texttt{\lit{hasEdge}(edge,acc,fp,fn)} & query & has edge & \lit{thr-query}(\syn{edge},\syn{ds},1,acc,fp,fn)\\\hline
\end{tabular}
\vspace{5pt}
\caption{Knowledge graph API and \tool{} specification fragments. The \texttt{VarExpr}, \texttt{VarExpr'}, and \texttt{VarExpr''} are \tool{} concept, relation, and interaction abstract HD variables expressions from the grammar in Figure~\ref{fig:grammar:speclang}. \texttt{N} is the degree of the graph. The \texttt{acc}, \texttt{fp}, \texttt{fn} rates are the accuracy, false positive, and false negative rates for the query respectively.}
\label{table:ds:knowledge}
\end{table}

We present a novel HD analysis-amenable knowledge graph representation that maintains per-node edge lists in item memory. A knowledge graph is a directed, labelled graph. Edges are labeled with codes from the relations codebook \codein{VarExpr'} and nodes are uniquely identified by codes from the concept codebook \codein{VarExpr}. The direction of each edge is indicated by an interaction code (\codein{VarExpr''}). Figure~\ref{table:ds:knowledge} presents the knowledge graph API and the \tool{} specification fragment associated with each API endpoint. The API supports creating knowledge graphs, adding nodes and edges to knowledge graphs, and filtering the nodes in the knowledge graph by an edge:

\begin{itemize}[leftmargin=*]
\item{}\textbf{Constructor (\texttt{\lit{KG}}).} The constructor specifies the maximum degree of the graph.
\item{}\textbf{Adding Vertices and Edges (\texttt{\lit{addVertex}}).} This API adds a vertex with its incident edge list to the graph.
\item{}\textbf{Querying Edges (\texttt{\lit{hasEdge}}).} This API specifies an edge query with accuracy requirements.
\end{itemize}

\subsubsection{Set Data Structure}\label{sec:datastructure:set}
\begin{table}[t]
\footnotesize
\setlength{\tabcolsep}{1.5pt}
\begin{tabular}{lllp{7cm}}
\textbf{Set / API call} & \textbf{type} & \textbf{description} & \textbf{\tool{} specification fragment}\\
\hline
\texttt{\lit{Set}(M,VarExpr)} & ctor & instantiate set & \texttt{\syn{ds} = \lit{sum}(M,VarExpr)}\\
\texttt{\lit{add}(query)} & modify & add element & \\
\texttt{\lit{inSet}(query,acc,fp,fn)} & query & element in set & \texttt{\lit{thr-query}(VarExpr,\syn{ds},1,acc,fp,fn)}\\
\texttt{\lit{subset}(query,M',K,acc,fp,fn)} & query & subset in set & 
\texttt{\lit{thr-query}(\lit{sum}(M',VarExpr),\syn{ds},K,acc,fp,fn)}\\
&&&\texttt{\lit{thr-query}(\lit{sum}(M'-1,VarExpr),\syn{ds},K,acc,fp,fn)}\\
&&&\texttt{...}\\
&&&\texttt{\lit{thr-query}(\lit{sum}(K,VarExpr),\syn{ds},K,acc,fp,fn)}\\
\hline

\end{tabular}
\caption{Set API and \tool{} specification fragments. \codein{VarExpr} is a \tool{} abstract HD expression from the grammar, \codein{query} is a concrete HD expression in \codein{VarExpr}, \codein{M} is the maximum size of the Set data structure, \codein{M'} is the maximum size of the subset query, and \codein{K} is the number of subset elements to match. The \codein{acc}, \codein{fp}, \codein{fn} rates are the accuracy, false positive, and false negative rates bounds for the query respectively.}
\label{fig:datastruct:set}
\end{table}

Figure~\ref{fig:datastruct:set} presents the analysis-amenable set data structure API endpoints and corresponding \tool{} specification fragments. The Set constructor instantiates the abstract data structure in the \tool{} specification, and the data structure queries introduce accuracy requirements into the specification.

\begin{itemize}[leftmargin=*]
\item{}\textbf{Constructor (\texttt{\lit{Set}}).} The constructor specifies the maximum number of elements in the set.
\item{}\textbf{Adding Elements (\texttt{\lit{add}}).} This API adds an element into the set.
\item{}\textbf{Querying if Elements in Set (\texttt{\lit{inSet}}).} This API specifies a single-element membership query with accuracy requirements.
\item{}\textbf{Querying if Subset in Set (\texttt{\lit{subset}}).} This API specifies a subset-set query with accuracy requirements.
\end{itemize}

% \noindent\textbf{Validity Checks.} The Set data structure ensures that all elements are members of the abstract HD expression \codein{VarExpr} provided to the set constructor. The Set data structure also ensures all elements in the set are mutually independent -- this constraint is imposed by the \tool{} analysis.

% \noindent\textbf{Hypervector and Query Optimization.} The data structure writes a single hypervector to item memory with the optimal hypervector size returned by the \tool{} static optimizer. Each query with an optimal query-specific threshold $\threshold_q$ and size $\hvsize_q$ is lowered to a $\hvsize_q$ dimensional hypervector. The distance is then partially computed over the first $\hvsize_q$ bits of the hypervector and compared with the query threshold $\threshold_q$. For subset queries, the data structure looks up the appropriate threshold and query size for the subset size.

\subsubsection{Analogical Database Data Structure}\label{sec:datastructure:database}

\begin{table}[t]
\footnotesize
\setlength{\tabcolsep}{1.5pt}
\begin{tabular}{lllp{6cm}}
\textbf{Database / API call} & \textbf{type} & \textbf{description} & \textbf{\tool{} specification fragment}\\
\hline
\texttt{\lit{Database}(M,VarExpr,VarExpr')} & ctor & create database & \texttt{\syn{kv} = \lit{prod}(VarExpr,VarExpr')} \\
& & & \texttt{\syn{ds} = \lit{sum}(M,\syn{kv})}\\
& & & \texttt{\syn{ds2} = \lit{prod}(\syn{ds},\syn{ds})}\\
& & & \texttt{\syn{val2} = \lit{prod}(VarExpr',VarExpr')}\\
%\texttt{\lit{addRecord(i)}} & modify & add record &  \\
%\texttt{\lit{addEntry(i,entry)}} & modify & add key-value to record &  \\
\texttt{\lit{addRecord(entries)}} & modify & add record &  \\
\texttt{\lit{matches}(pairs,M',K,acc,fp,fn)} & query & find records with $\geq$ K & \texttt{\lit{thr-query}(\lit{sum}(M',\syn{kv}),\syn{ds},K,acc,fp,fn)}\\
&& query tuple matches&\texttt{\lit{thr-query}(\lit{sum}(M'-1,\syn{kv}),\syn{ds},K,acc,fp,fn)}\\
&&&...\\
&&&\texttt{\lit{thr-query}(\lit{sum}(K,\syn{kv}),\syn{ds},K,acc,fp,fn)}\\
\texttt{\lit{analogy}(query,m,acc,t,prob)} & query & analogical query& \texttt{\lit{wta-query}(\syn{val2},\syn{ds2},1,1,m,acc,t,prob)}\\\hline

\end{tabular}
\caption{Analogical Database API and \tool{} specification fragments. \codein{VarExpr} and \codein{VarExpr'} are \tool{} key and value abstract HD variables expressions from the grammar, \codein{ds} is a set of (VarExpr,VarExpr') tuples, representing records, \codein{query} is a tuple of two values. The value \codein{M} is the maximum length of a record, \codein{M'} is the maximum length of the queried record in match queries, and \codein{K} is the number of entries to match. \codein{m} in the analogy query is the number of distinct values in item memory.}
\label{fig:datastruct:database}
\end{table}

Karnerva~\cite{kanerva2010we} presented a specialized database query that leverages hyperdimensional computing to compute mappings between analogical structures that can be effectively conducted via HDC. The classic example of such a query is the "dollar price of mexico" query in which each database record is queried to fill in the analogy \codein{us:dollar} as \codein{mexico:?}. 

Figure~\ref{fig:datastruct:database} presents an analysis-amenable analogical database data structure that stores individual database records in item memory. Each database record is a hypervector that encodes a set containing up to \codein{M} key-value tuples, where each key-value tuple is a member of \codein{\lit{prod}(VarExpr,VarExpr')}. The \codein{matches} API call finds the records that match at least \codein{K} of the key-value pairs in \codein{pairs}, and the \codein{analogy} query retrieves the value in the record that completes the analogical query \codein{query}.

\begin{itemize}[leftmargin=*]
\item{}\textbf{Constructor (\texttt{\lit{Database}}).} The constructor specifies the maximum length (number of entries) of a record in database.
\item{}\textbf{Adding Elements (\texttt{\lit{addRecord}}).} This API adds a record with specified entries to the database.
\item{}\textbf{Database Queries (\texttt{\lit{matches}}).} This API specifies a match query, with the maximum length of the queried record, the number of entries to match and accuracy requirements.
\item{}\textbf{Analogical Database Queries (\texttt{\lit{analogy}}).} This API specifies a winner-take-all analogy query, with the maximum number of distinct values, and the required hard and soft accuracy constraints.
\end{itemize}

% \noindent\textbf{Validity Checks.} The data structure checks that no key is bound more than once in a single record, and validates the tuples in each record set are mutually independent -- this constraint is imposed by the \tool{} analysis. 

% \noindent\textbf{Hypervector Optimization.} the width of the record hypervectors stored in memory are set to the optimal hypervector size. Each database query is configured to use the query-specific threshold and query hypervector size. The \codein{matches} queries are specialized to use the threshold and size that corresponds to the the number of elements in the query set.

\subsubsection{Non-Deterministic Finite Automata}\label{sec:datastructure:nfa}

\begin{table}[t]
\footnotesize
\setlength{\tabcolsep}{1.5pt}
\begin{tabular}{lllp{6cm}}
\textbf{NFA / API call} & \textbf{type} & \textbf{description} & \textbf{\tool{} specification fragment}\\
\hline
\texttt{\lit{NFA}(N,M,VarExpr,VarExpr')} & ctor & NFA instantiation & \texttt{\syn{states} = \lit{sum}(N,VarExpr)}\\
& & & \texttt{\syn{trans} = \lit{prod}(VarExpr,VarExpr',\lit{perm}(1,VarExpr))}\\
& & & \texttt{\syn{nfa} = \lit{sum}(M,\syn{trans})}\\
\texttt{\lit{setNFA}(transitions)} & modify & set NFA transitions & \\
\texttt{\lit{startStates}(states)} & modify & set start states &\\
\texttt{\lit{execute}(sym,acc,fp,fn)} & modify/query & apply symbol & \texttt{\syn{states'} = \lit{perm}(-1,\lit{prod}(VarExpr',\syn{nfa},\syn{states}))}\\
& & & \texttt{\lit{thr-query}(VarExpr,\syn{states'},1,acc,fp,fn)}\\\hline
\end{tabular}
\caption{Non-deterministic Finite-State Automata (NFA) API and \tool{} specification fragments. The \codein{VarExpr} and \codein{VarExpr'} are \tool{} state and input symbols. \codein{N} is the maximum number of states. \codein{M} is the maximum number of transitions. NFA (\codein{nfa}) is described as a set of transitions.}
\label{table:ds:nfa}
\end{table}

Figure~\ref{table:ds:nfa} presents the API for an analysis-amenable non-deterministic finite automata that is built on the HD finite-state automata formulation developed by Pashchenko et al.~\cite{pashchenko2020search}. The NFA maintains a state hypervector over NFA state codes (\syn{states}) and transition hypervector over state-symbol-state tuples (\syn{nfa}). The permutation operator encodes the history of states. The API provides endpoints for instantiating an \codein{N}-state \codein{M}-transition NFA and for instantiating the NFA transitions and inital set of states. The \codein{\lit{execute}} endpoint applies a symbol to the NFA and computes the NFA's next set of states. The execution endpoint qualifies as a query because it ensure the current state can be accurately recovered from the state vector with accuracy \codein{acc}.
%To generate a \tool{} specification, the NFA execution calls need to be unrolled a fixed number of types.

\begin{itemize}[leftmargin=*]
\item{}\textbf{Constructor (\texttt{\lit{NFA}}).} The constructor specifies the maximum number of states, and maximum number of transitions.
\item{}\textbf{Setting up the NFA (\texttt{\lit{setNFA}}, \texttt{\lit{startStates}}).} These two APIs specify the transitions of the NFA, and the starting state set.
\item{}\textbf{Applying a State Transition (\texttt{\lit{execute}}).} This API execute the NFA on a given symbol \codein{sym}. It specifies the accuracy requirements for retrieving a new state set after the execution.
\end{itemize}

% \noindent\textbf{Validity Checks.} The NFA checks that the start state set is valid - it should only contain mutually independent state codes.

\noindent\textbf{Hypervector Optimizations at Runtime.} The NFA uses the optimal hypervector size for the state and transition hypervectors. The NFA uses the query size and threshold to successively query NFA states and rebuild a lower-noise state vector. This noise-reducing 'cleanup' operation enables the HD computational error to remain relatively controlled as the NFA continues execution. In the event the NFA has a monotonically decreasing set of states (e.g., for string matching~\cite{pashchenko2020search}), the size of the state vector is dynamically reduced using the query-specific dimension.

\subsubsection{Data Structure Optimizations at Runtime}\label{sec:datastructure:optimizations}

\noindent\textit{Using Heim-Optimized Parameters.} \tool{} returns the minimum hypervector size that delivers the desired accuracy requirements, and a set of optimal query parameters for each query accuracy constraint:

\begin{itemize}
\item\textbf{Threshold-Based Queries}(\codein{thr-query(Expr,Expr',k,x,x',x'')}) For each threshold-based query, \tool{} returns collection of distance thresholds to use for each query retrieving 1..$k$ elements. \tool{} also returns the minimum hypervector size needed to complete the query with the desired accuracy.

\item\textbf{Winner-Take-All Queries}(\codein{wta-query(Expr,Expr',k,w,m,x,t,x')}) For each WTA query, \tool{} returns the minimum hypervector size needed to complete the query with the desired accuracy.
\end{itemize}

For each data structure, the data structure's hypervector dimension is set to the optimal hypervector size, and the optimal distance thresholds are used to complete each threshold based query. The query-specific optimal hypervector size is used to perform sound partial computation of the hypervector distance.
